# Supplementary material for: Exponentially Stable Adaptive Optimal Control of Uncertain LTI Systems
Source: arXiv:2205.02913 ancillary file (2023-08-21)
Supplement: Supplementary file 1 [file supp.pdf]

Received: Added at production | Revised: Added at production | Accepted: Added at production

DOI: xxx/xxxx

SUPPLEMENTARY MATERIAL

# Supplement to "Exponentially Stable Adaptive Optimal Control of Uncertain LTI Systems"

Anton Glushchenko* | Konstantin Lastochkin

[1]Ya.Z. Tsypkin Laboratory of Adaptive and Robust Systems, V.A. Trapeznikov Institute of Control Sciences of Russian Academy of Sciences, Moscow, Russia

**Correspondence**
*Anton Glushchenko, Russia, Moscow, Profsoyuznaya street, h.65, 117997, ICS RAS. Email: aiglush@ipu.ru

**Summary**

This article is the supplementary material for the research paper 'Exponentially Stable Adaptive Optimal Control of Uncertain LTI Systems'. It gives more details on how to obtain the equations (14), (A6) and (A7) and is being referred in appropriate places in the paper.

## 1 | EXPLANATION ON HOW TO OBTAIN EQUATION (14) IN THE MANUSCRIPT

First of all, let the first line of the equation (14) from the manuscript be presented:

$$\begin{gathered}\tilde{J} = \hat{J} - J = \tfrac{1}{2}\int\limits_{t_r^+}^{\infty} x^{\mathrm{T}}(t)\,Qx(t) + u^{\mathrm{T}}(t)\,Ru(t)\,dt - \\ -\tfrac{1}{2}\int\limits_{t_r^+}^{\infty} x_{ref}^{\mathrm{T}}(t)\,Qx_{ref}(t) + (u^*)^{\mathrm{T}}(t)\,Ru^*(t)\,dt\end{gathered} \tag{S1}$$

Then the following axillary equations are introduced:

$$\begin{gathered}x^{\mathrm{T}}(t)\,Qx(t) - x_{ref}^{\mathrm{T}}(t)\,Qx_{ref}(t) = \\ = \left(e_{ref}(t) + x_{ref}(t)\right)^{\mathrm{T}} Q\left(e_{ref}(t) + x_{ref}(t)\right) - x_{ref}^{\mathrm{T}}(t)\,Qx_{ref}(t) = \\ = e_{ref}^{\mathrm{T}}(t)\,Qe_{ref}(t) + e_{ref}^{\mathrm{T}}(t)\,Qx_{ref}(t) + x_{ref}^{\mathrm{T}}(t)\,Qe_{ref}(t)\end{gathered} \tag{S2}$$

$$\begin{gathered}u^{\mathrm{T}}(t)\,Ru(t) - (u^*)^{\mathrm{T}}(t)\,Ru^*(t) = \omega^{\mathrm{T}}(t)\,\hat{\theta}R\hat{\theta}^{\mathrm{T}}\omega(t) - \omega^{\mathrm{T}}(t)\,\theta R\theta^{\mathrm{T}}\omega(t) = \\ = \omega^{\mathrm{T}}(t)\left(\tilde{\theta} + \theta\right)R\hat{\theta}^{\mathrm{T}}\omega(t) - \omega^{\mathrm{T}}(t)\,\theta R\theta^{\mathrm{T}}\omega(t) = \\ = \omega^{\mathrm{T}}(t)\,\tilde{\theta}R\hat{\theta}^{\mathrm{T}}\omega(t) + \omega^{\mathrm{T}}(t)\,\theta R\left(\tilde{\theta} + \theta\right)^{\mathrm{T}}\omega(t) - \omega^{\mathrm{T}}(t)\,\theta R\theta^{\mathrm{T}}\omega(t) = \\ = \omega^{\mathrm{T}}(t)\,\tilde{\theta}R\left(\tilde{\theta} + \theta\right)^{\mathrm{T}}\omega(t) + \omega^{\mathrm{T}}(t)\,\theta R\tilde{\theta}^{\mathrm{T}}\omega(t) = \\ = \omega^{\mathrm{T}}(t)\,\tilde{\theta}R\tilde{\theta}^{\mathrm{T}}\omega(t) + \omega^{\mathrm{T}}(t)\,\tilde{\theta}R\theta^{\mathrm{T}}\omega(t) + \omega^{\mathrm{T}}(t)\,\theta R\tilde{\theta}^{\mathrm{T}}\omega(t)\end{gathered} \tag{S3}$$

Substituting (S2) and (S3) into (S1), the equation (14) in the manuscript is obtained:

$$\begin{gathered}\tilde{J} = \hat{J} - J = \tfrac{1}{2}\int\limits_{t_r^+}^{\infty} x^{\mathrm{T}}(t)\,Qx(t) + u^{\mathrm{T}}(t)\,Ru(t)\,dt - \\ -\tfrac{1}{2}\int\limits_{t_r^+}^{\infty} x_{ref}^{\mathrm{T}}(t)\,Qx_{ref}(t) + (u^*)^{\mathrm{T}}(t)\,Ru^*(t)dt = \\ = \tfrac{1}{2}\int\limits_{t_r^+}^{\infty} e_{ref}^{\mathrm{T}}(t)\,Qe_{ref}(t) + e_{ref}^{\mathrm{T}}(t)\,Qx_{ref}(t) + x_{ref}^{\mathrm{T}}(t)\,Qe_{ref}(t)\,dt + \\ +\tfrac{1}{2}\int\limits_{t_r^+}^{\infty} \omega^{\mathrm{T}}(t)\,\tilde{\theta}(t)\,R\tilde{\theta}^{\mathrm{T}}(t)\,\omega(t) + \omega^{\mathrm{T}}(t)\,\tilde{\theta}(t)\,R\theta^{\mathrm{T}}\omega(t) + \omega^{\mathrm{T}}(t)\,\theta R\tilde{\theta}^{\mathrm{T}}(t)\,\omega(t)\,dt\end{gathered} \tag{S4}$$

## 2 | EXPLANATION ON HOW TO OBTAIN EQUATIONS (A6) AND (A7) IN THE MANUSCRIPT

First of all, the equation (A6) in the manuscript is considered. The following is to be taken into consideration:

$$\begin{array}{c} y_{K_x}(t) = \Delta_{K_x}(t) K_x + \varepsilon_{K_x}(t), \\ z_{\Phi_{11}}(t) - \varepsilon_{\Phi_{11}}(t) := \Delta_{\Phi}(t) \Phi_{11}(\tau), \\ z_{\Phi_{21}}(t) - \varepsilon_{\Phi_{21}}(t) := \Delta_{\Phi}(t) \Phi_{21}(\tau). \end{array} \tag{S5}$$

Then $y_{K_x}(t)$ is written as follows:

$$\begin{array}{c} y_{K_x}(t) := -\Delta_{\Phi}^{n}(t) \varphi(t) R^{-1} B^{\mathrm{T}} \Phi_{21}\left(\tau_{\infty}\right) adj\left\{\Phi_{11}\left(\tau_{\infty}\right)\right\} = \\ = -\Delta_{\Phi}^{n-1}(t) R^{-1} z_B^{\mathrm{T}}(t) \Delta_{\Phi}(t) \Phi_{21}\left(\tau_{\infty}\right) adj\left\{\Phi_{11}\left(\tau_{\infty}\right)\right\} = \\ = -R^{-1} z_B^{\mathrm{T}}(t) \Delta_{\Phi}(t) \Phi_{21}\left(\tau_{\infty}\right) adj\left\{\Delta_{\Phi}(t) \Phi_{11}\left(\tau_{\infty}\right)\right\} = \\ = -R^{-1} z_B^{\mathrm{T}}(t)\left(z_{\Phi_{21}}(t) - \varepsilon_{\Phi_{21}}(t)\right) adj\left\{z_{\Phi_{11}}(t) - \varepsilon_{\Phi_{11}}(t)\right\} = \\ = -R^{-1} z_B^{\mathrm{T}}(t) z_{\Phi_{21}}(t) adj\left\{z_{\Phi_{11}}(t)\right\} - R^{-1} z_B^{\mathrm{T}}(t) z_{\Phi_{21}}(t) adj\left\{-\varepsilon_{\Phi_{11}}(t)\right\} + \\ + R^{-1} z_B^{\mathrm{T}}(t) \varepsilon_{\Phi_{21}}(t) adj\left\{z_{\Phi_{11}}(t) - \varepsilon_{\Phi_{11}}(t)\right\} \end{array} \tag{S6}$$

The first summond in (S6) is $y_{K_x}(t)$ exactly, whereas the second one will be used to form $\varepsilon_{K_x}(t)$. The equation for $\Delta_{K_x}(t)$ is transformed in the same way:

$$\begin{array}{c} \Delta_{K_x}(t) := \Delta_{\Phi}^{n}(t) \varphi(t) \det\left\{\Phi_{11}\left(\tau_{\infty}\right)\right\} = \varphi(t) \det\left\{\Delta_{\Phi}(t) \Phi_{11}\left(\tau_{\infty}\right)\right\} = \\ = \varphi(t) \det\left\{\Delta_{\Phi}(t) \Phi_{11}\left(\tau_{\infty}\right)\right\} \pm \varphi(t) \det\left\{z_{\Phi_{11}}(t)\right\} = \\ = \varphi(t) \det\left\{z_{\Phi_{11}}(t)\right\} + \varphi(t)\left(\det\left\{\Delta_{\Phi}(t) \Phi_{11}\left(\tau_{\infty}\right)\right\} - \det\left\{z_{\Phi_{11}}(t)\right\}\right). \end{array} \tag{S7}$$

And again, the first summond in (S7) is $\Delta_{K_x}(t)$ exactly, whereas the second one will be used to form $\varepsilon_{K_x}(t)$.

So, considering (S1), the following equations could be written:

$$\begin{array}{c} y_{K_x}(t) := -R^{-1} z_B^{\mathrm{T}}(t) z_{\Phi_{21}}(t) adj\left\{z_{\Phi_{11}}(t)\right\}, \\ \Delta_{K_x}(t) := \varphi(t) \det\left\{z_{\Phi_{11}}(t)\right\}, \\ \varepsilon_{K_x}(t) := R^{-1} z_B^{\mathrm{T}}(t) z_{\Phi_{21}}(t) adj\left\{-\varepsilon_{\Phi_{11}}(t)\right\} - \\ -R^{-1} z_B^{\mathrm{T}}(t) \varepsilon_{\Phi_{21}}(t) adj\left\{z_{\Phi_{11}}(t) - \varepsilon_{\Phi_{11}}(t)\right\} + \\ +\varphi(t)\left(\det\left\{\Delta_{\Phi}(t) \Phi_{11}\left(\tau_{\infty}\right)\right\} - \det\left\{z_{\Phi_{11}}(t)\right\}\right) K_x, \end{array} \tag{S8}$$

which are exactly the final equations of $y_{K_x}(t)$, $\Delta_{K_x}(t)$ and $\varepsilon_{K_x}(t)$ in (A6) in the manuscript.

Let the equation (A7) be considered. The following is to be taken into consideration:

$$y_{K_r}(t) = \Delta_{K_r} K_r(t) + \varepsilon_{K_r}(t). \tag{S9}$$

Then $y_{K_r}(t)$ is written as follows (we have omitted the speculations, which are shown in (A7) in the manuscript before the sign $\stackrel{\Delta}{=}$ and denoted them as "..."):

$$\begin{array}{c}
y_{K_r}(t) = \varphi^{2n}(t)\,\Delta_{\Phi}^{n^2}(t)\,y_{K_r} = \ldots = \\
-\varphi(t)\,R^{-1}z_B^{\mathrm{T}}(t)\times \\
\times adj\left\{\begin{array}{l} \varphi(t)\,z_A^{\mathrm{T}}(t)\det\left\{\Delta_{\Phi}(t)\,\Phi_{11}\left(\tau_\infty\right)\right\} - \Delta_{\Phi}(t)\,\Phi_{21}\left(\tau_\infty\right)\times \\ \times adj\left\{\Delta_{\Phi}(t)\,\Phi_{11}\left(\tau_\infty\right)\right\}z_B(t)\,R^{-1}z_B^{\mathrm{T}}(t)\end{array}\right\}\times \\
\times\Delta_{\Phi}(t)\,\Phi_{21}\left(\tau_\infty\right)adj\left\{\Delta_{\Phi}(t)\,\Phi_{11}\left(\tau_\infty\right)\right\}B_r = \\
= -\varphi(t)\,R^{-1}z_B^{\mathrm{T}}(t)\times \\
\times adj\left\{\begin{array}{l} \varphi(t)\,z_A^{\mathrm{T}}(t)\det\left\{\Delta_{\Phi}(t)\,\Phi_{11}\left(\tau_\infty\right)\right\} - \Delta_{\Phi}(t)\,\Phi_{21}\left(\tau_\infty\right)\times \\ \times adj\left\{\Delta_{\Phi}(t)\,\Phi_{11}\left(\tau_\infty\right)\right\}z_B(t)\,R^{-1}z_B^{\mathrm{T}}(t)\end{array}\right\}\times \\
\times\Delta_{\Phi}(t)\,\Phi_{21}\left(\tau_\infty\right)adj\left\{\Delta_{\Phi}(t)\,\Phi_{11}\left(\tau_\infty\right)\right\}B_r = \\
\left[\begin{array}{c}
= -\varphi(t)\,R^{-1}z_B^{\mathrm{T}}(t)\times \\
\times adj\left\{\begin{array}{l} \varphi(t)\,z_A^{\mathrm{T}}(t)\det\left\{\Delta_{\Phi}(t)\,\Phi_{11}\left(\tau_\infty\right)\right\} - \\ -\Delta_{\Phi}(t)\,\Phi_{21}\left(\tau_\infty\right)adj\left\{\Delta_{\Phi}(t)\,\Phi_{11}\left(\tau_\infty\right)\right\}z_B(t)\,R^{-1}z_B^{\mathrm{T}}(t)\end{array}\right\}\times \\
\times\left(z_{\Phi_{21}}(t) - \varepsilon_{\Phi_{21}}(t)\right)adj\left\{\Delta_{\Phi}(t)\,\Phi_{11}\left(\tau_\infty\right)\right\}B_r =
\end{array}\right] \\
= \varphi(t)\,R^{-1}z_B^{\mathrm{T}}(t)\times \\
\times adj\left\{\begin{array}{l} \varphi(t)\,z_A^{\mathrm{T}}(t)\det\left\{\Delta_{\Phi}(t)\,\Phi_{11}\left(\tau_\infty\right)\right\} - \\ -\Delta_{\Phi}(t)\,\Phi_{21}\left(\tau_\infty\right)adj\left\{\Delta_{\Phi}(t)\,\Phi_{11}\left(\tau_\infty\right)\right\}z_B(t)\,R^{-1}z_B^{\mathrm{T}}(t)\end{array}\right\}\times \\
\times\varepsilon_{\Phi_{21}}(t)\,adj\left\{\Delta_{\Phi}(t)\,\Phi_{11}\left(\tau_\infty\right)\right\}B_r - \\
\left[\begin{array}{c}
-\varphi(t)\,R^{-1}z_B^{\mathrm{T}}(t)\times \\
\times adj\left\{\begin{array}{l} \varphi(t)\,z_A^{\mathrm{T}}(t)\det\left\{\Delta_{\Phi}(t)\,\Phi_{11}\left(\tau_\infty\right)\right\} - \\ -\Delta_{\Phi}(t)\,\Phi_{21}\left(\tau_\infty\right)adj\left\{\Delta_{\Phi}(t)\,\Phi_{11}\left(\tau_\infty\right)\right\}z_B(t)\,R^{-1}z_B^{\mathrm{T}}(t)\end{array}\right\}\times \\
\times z_{\Phi_{21}}(t)\,adj\left\{z_{\Phi_{11}}(t) - \varepsilon_{\Phi_{11}}(t)\right\}B_r =
\end{array}\right] \\
= \varphi(t)\,R^{-1}z_B^{\mathrm{T}}(t)\times \\
\times adj\left\{\begin{array}{l} \varphi(t)\,z_A^{\mathrm{T}}(t)\det\left\{\Delta_{\Phi}(t)\,\Phi_{11}\left(\tau_\infty\right)\right\} - \\ -\Delta_{\Phi}(t)\,\Phi_{21}\left(\tau_\infty\right)adj\left\{\Delta_{\Phi}(t)\,\Phi_{11}\left(\tau_\infty\right)\right\}z_B(t)\,R^{-1}z_B^{\mathrm{T}}(t)\end{array}\right\}\times \\
\times\varepsilon_{\Phi_{21}}(t)\,adj\left\{\Delta_{\Phi}(t)\,\Phi_{11}\left(\tau_\infty\right)\right\}B_r - \\
-\varphi(t)\,R^{-1}z_B^{\mathrm{T}}(t)\times \\
\times adj\left\{\begin{array}{l} \varphi(t)\,z_A^{\mathrm{T}}(t)\det\left\{\Delta_{\Phi}(t)\,\Phi_{11}\left(\tau_\infty\right)\right\} - \\ -\Delta_{\Phi}(t)\,\Phi_{21}\left(\tau_\infty\right)adj\left\{\Delta_{\Phi}(t)\,\Phi_{11}\left(\tau_\infty\right)\right\}z_B(t)\,R^{-1}z_B^{\mathrm{T}}(t)\end{array}\right\}\times \\
\times z_{\Phi_{21}}(t)\,adj\left\{-\varepsilon_{\Phi_{11}}(t)\right\}B_r - \\
\left[\begin{array}{c}
-\varphi(t)\,R^{-1}z_B^{\mathrm{T}}(t)\times \\
\times adj\left\{\begin{array}{l} \varphi(t)\,z_A^{\mathrm{T}}(t)\det\left\{\Delta_{\Phi}(t)\,\Phi_{11}\left(\tau_\infty\right)\right\} - \left(z_{\Phi_{21}}(t) - \varepsilon_{\Phi_{21}}(t)\right)\times \\ \times adj\left\{\Delta_{\Phi}(t)\,\Phi_{11}\left(\tau_\infty\right)\right\}z_B(t)\,R^{-1}z_B^{\mathrm{T}}(t)\end{array}\right\}\times \\
\times z_{\Phi_{21}}(t)\,adj\left\{z_{\Phi_{11}}(t)\right\}B_r =
\end{array}\right]
\end{array} \tag{S10}$$

$$
\begin{gathered}
= +\varphi(t) R^{-1} z_B^{\mathrm{T}}(t) \times \\
\times adj \left\{ \begin{gathered} \varphi(t) z_A^{\mathrm{T}}(t) \det\left\{\Delta_\Phi(t)\Phi_{11}\left(\tau_\infty\right)\right\} - \\ -\Delta_\Phi(t)\Phi_{21}\left(\tau_\infty\right) adj\left\{\Delta_\Phi(t)\Phi_{11}\left(\tau_\infty\right)\right\} z_B(t) R^{-1} z_B^{\mathrm{T}}(t) \end{gathered} \right\} \times \\
\times \varepsilon_{\Phi_{21}}(t)\, adj\left\{\Delta_\Phi(t)\Phi_{11}\left(\tau_\infty\right)\right\} B_r - \\
-\varphi(t) R^{-1} z_B^{\mathrm{T}}(t) \times \\
\times adj \left\{ \begin{gathered} \varphi(t) z_A^{\mathrm{T}}(t) \det\left\{\Delta_\Phi(t)\Phi_{11}\left(\tau_\infty\right)\right\} - \\ -\Delta_\Phi(t)\Phi_{21}\left(\tau_\infty\right) adj\left\{\Delta_\Phi(t)\Phi_{11}\left(\tau_\infty\right)\right\} z_B(t) R^{-1} z_B^{\mathrm{T}}(t) \end{gathered} \right\} \times \\
\times z_{\Phi_{21}}(t)\, adj\left\{-\varepsilon_{\Phi_{11}}(t)\right\} B_r - \\
-\varphi(t) R^{-1} z_B^{\mathrm{T}}(t) \times \\
\times adj\left\{\varepsilon_{\Phi_{21}}(t)\, adj\left\{\Delta_\Phi(t)\Phi_{11}\left(\tau_\infty\right)\right\} z_B(t) R^{-1} z_B^{\mathrm{T}}(t)\right\} z_{\Phi_{21}}(t)\, adj\left\{z_{\Phi_{11}}(t)\right\} B_r - \\
\left[ \begin{gathered} -\varphi(t) R^{-1} z_B^{\mathrm{T}}(t) \times \\ \times adj \left\{ \begin{gathered} \varphi(t) z_A^{\mathrm{T}}(t) \det\left\{\Delta_\Phi(t)\Phi_{11}\left(\tau_\infty\right)\right\} - \\ -z_{\Phi_{21}}(t)\, adj\left\{z_{\Phi_{11}}(t) - \varepsilon_{\Phi_{11}}(t)\right\} z_B(t) R^{-1} z_B^{\mathrm{T}}(t) \end{gathered} \right\} \times \\ \times z_{\Phi_{21}}(t)\, adj\left\{z_{\Phi_{11}}(t)\right\} B_r = \end{gathered} \right] \\
= +\varphi(t) R^{-1} z_B^{\mathrm{T}}(t) \times \\
\times adj \left\{ \begin{gathered} \varphi(t) z_A^{\mathrm{T}}(t) \det\left\{\Delta_\Phi(t)\Phi_{11}\left(\tau_\infty\right)\right\} - \\ -\Delta_\Phi(t)\Phi_{21}\left(\tau_\infty\right) adj\left\{\Delta_\Phi(t)\Phi_{11}\left(\tau_\infty\right)\right\} z_B(t) R^{-1} z_B^{\mathrm{T}}(t) \end{gathered} \right\} \times \\
\times \varepsilon_{\Phi_{21}}(t)\, adj\left\{\Delta_\Phi(t)\Phi_{11}\left(\tau_\infty\right)\right\} B_r - \\
-\varphi(t) R^{-1} z_B^{\mathrm{T}}(t) \times \\
\times adj \left\{ \begin{gathered} \varphi(t) z_A^{\mathrm{T}}(t) \det\left\{\Delta_\Phi(t)\Phi_{11}\left(\tau_\infty\right)\right\} - \\ -\Delta_\Phi(t)\Phi_{21}\left(\tau_\infty\right) adj\left\{\Delta_\Phi(t)\Phi_{11}\left(\tau_\infty\right)\right\} z_B(t) R^{-1} z_B^{\mathrm{T}}(t) \end{gathered} \right\} \times \\
\times z_{\Phi_{21}}(t)\, adj\left\{-\varepsilon_{\Phi_{11}}(t)\right\} B_r - \\
-\varphi(t) R^{-1} z_B^{\mathrm{T}}(t) \times \\
\times adj\left\{\varepsilon_{\Phi_{21}}(t)\, adj\left\{\Delta_\Phi(t)\Phi_{11}\left(\tau_\infty\right)\right\} z_B(t) R^{-1} z_B^{\mathrm{T}}(t)\right\} z_{\Phi_{21}}(t)\, adj\left\{z_{\Phi_{11}}(t)\right\} B_r - \\
-\varphi(t) R^{-1} z_B^{\mathrm{T}}(t)\, adj\left\{-z_{\Phi_{21}}(t)\, adj\left\{-\varepsilon_{\Phi_{11}}(t)\right\} z_B(t) R^{-1} z_B^{\mathrm{T}}(t)\right\} z_{\Phi_{21}}(t)\, adj\left\{z_{\Phi_{11}}(t)\right\} B_r - \\
\left[ \begin{gathered} -\varphi(t) R^{-1} z_B^{\mathrm{T}}(t) \times \\ \times adj \left\{ \begin{gathered} \varphi(t) z_A^{\mathrm{T}}(t) \det\left\{z_{\Phi_{11}}(t) - \varepsilon_{\Phi_{11}}(t)\right\} \pm \varphi(t) z_A^{\mathrm{T}}(t) \det\left\{z_{\Phi_{11}}(t)\right\} \\ -z_{\Phi_{21}}(t)\, adj\left\{z_{\Phi_{11}}(t)\right\} z_B(t) R^{-1} z_B^{\mathrm{T}}(t) \end{gathered} \right\} \times \\ \times z_{\Phi_{21}}(t)\, adj\left\{z_{\Phi_{11}}(t)\right\} B_r = \end{gathered} \right] \\
= +\varphi(t) R^{-1} z_B^{\mathrm{T}}(t) \times \\
\times adj \left\{ \begin{gathered} \varphi(t) z_A^{\mathrm{T}}(t) \det\left\{\Delta_\Phi(t)\Phi_{11}\left(\tau_\infty\right)\right\} - \\ -\Delta_\Phi(t)\Phi_{21}\left(\tau_\infty\right) adj\left\{\Delta_\Phi(t)\Phi_{11}\left(\tau_\infty\right)\right\} z_B(t) R^{-1} z_B^{\mathrm{T}}(t) \end{gathered} \right\} \times \\
\times \varepsilon_{\Phi_{21}}(t)\, adj\left\{\Delta_\Phi(t)\Phi_{11}\left(\tau_\infty\right)\right\} B_r - \\
-\varphi(t) R^{-1} z_B^{\mathrm{T}}(t) \times \\
\times adj \left\{ \begin{gathered} \varphi(t) z_A^{\mathrm{T}}(t) \det\left\{\Delta_\Phi(t)\Phi_{11}\left(\tau_\infty\right)\right\} - \\ -\Delta_\Phi(t)\Phi_{21}\left(\tau_\infty\right) adj\left\{\Delta_\Phi(t)\Phi_{11}\left(\tau_\infty\right)\right\} z_B(t) R^{-1} z_B^{\mathrm{T}}(t) \end{gathered} \right\} \times \\
\times z_{\Phi_{21}}(t)\, adj\left\{-\varepsilon_{\Phi_{11}}(t)\right\} B_r - \\
-\varphi(t) R^{-1} z_B^{\mathrm{T}}(t) \times \\
\times adj\left\{\varepsilon_{\Phi_{21}}(t)\, adj\left\{\Delta_\Phi(t)\Phi_{11}\left(\tau_\infty\right)\right\} z_B(t) R^{-1} z_B^{\mathrm{T}}(t)\right\} z_{\Phi_{21}}(t)\, adj\left\{z_{\Phi_{11}}(t)\right\} B_r - \\
-\varphi(t) R^{-1} z_B^{\mathrm{T}}(t)\, adj\left\{-z_{\Phi_{21}}(t)\, adj\left\{-\varepsilon_{\Phi_{11}}(t)\right\} z_B(t) R^{-1} z_B^{\mathrm{T}}(t)\right\} z_{\Phi_{21}}(t)\, adj\left\{z_{\Phi_{11}}(t)\right\} B_r - \\
-\varphi(t) R^{-1} z_B^{\mathrm{T}}(t) \times \\
\times adj\left\{\varphi(t) z_A^{\mathrm{T}}(t) \left(\det\left\{z_{\Phi_{11}}(t) - \varepsilon_{\Phi_{11}}(t)\right\} - \det\left\{z_{\Phi_{11}}(t)\right\}\right)\right\} z_{\Phi_{21}}(t)\, adj\left\{z_{\Phi_{11}}(t)\right\} B_r - \\
\left[ \begin{gathered} -\varphi(t) R^{-1} z_B^{\mathrm{T}}(t) \times \\ \times adj \left\{ \begin{gathered} \varphi(t) z_A^{\mathrm{T}}(t) \det\left\{z_{\Phi_{11}}(t)\right\} - \\ -z_{\Phi_{21}}(t)\, adj\left\{z_{\Phi_{11}}(t)\right\} z_B(t) R^{-1} z_B^{\mathrm{T}}(t) \end{gathered} \right\} \times \\ \times z_{\Phi_{21}}(t)\, adj\left\{z_{\Phi_{11}}(t)\right\} B_r \end{gathered} \right]
\end{gathered}
$$

Considering the final expression of $y_{K_r}(t)$, the summonds highlighted in blue are $y_{K_r}(t)$ exactly, whereas the ones highlighted in red will be used to form $\varepsilon_{K_r}(t)$.

The next step is to write the expression for $\Delta_{K_r}(t)$ (we have omitted the speculations, which are shown in (A7) in the manuscript before the sign $\overset{\Delta}{=}$ and denoted them as "..."):

$$
\begin{array}{c}
\Delta_{K_r}(t) = \varphi^{2n}(t)\,\Delta_{\Phi}^{n^2}(t)\,\Delta_V\,\Delta_P^n = \ldots = \\
= \det\left\{ \begin{array}{c} \det\left\{\Delta_\Phi(t)\,\Phi_{11}\left(\tau_\infty\right)\right\}\varphi(t)\,z_A^{\mathrm{T}}(t) - \\ -\Delta_\Phi(t)\,\Phi_{21}\left(\tau_\infty\right) adj\left\{\Delta_\Phi(t)\,\Phi_{11}\left(\tau_\infty\right)\right\} z_B(t)\,R^{-1}z_B^{\mathrm{T}}(t) \end{array} \right\} = \\
= \det\left\{ \begin{array}{c} \det\left\{\Delta_\Phi(t)\,\Phi_{11}\left(\tau_\infty\right)\right\}\varphi(t)\,z_A^{\mathrm{T}}(t) - \\ -\left(z_{\Phi_{21}}(t) - \varepsilon_{\Phi_{21}}(t)\right) adj\left\{\Delta_\Phi(t)\,\Phi_{11}\left(\tau_\infty\right)\right\} z_B(t)\,R^{-1}z_B^{\mathrm{T}}(t) \end{array} \right\} = \\
= \det\left\{ \begin{array}{c} \det\left\{\Delta_\Phi(t)\,\Phi_{11}\left(\tau_\infty\right)\right\}\varphi(t)\,z_A^{\mathrm{T}}(t) - \\ -z_{\Phi_{21}}(t)\,adj\left\{z_{\Phi_{11}}(t) - \varepsilon_{\Phi_{11}}(t)\right\} z_B(t)\,R^{-1}z_B^{\mathrm{T}}(t) + \\ +\varepsilon_{\Phi_{21}}(t)\,adj\left\{\Delta_\Phi(t)\,\Phi_{11}\left(\tau_\infty\right)\right\} z_B(t)\,R^{-1}z_B^{\mathrm{T}}(t) \end{array} \right\} = \\
= \det\left\{ \begin{array}{c} \left(\det\left\{z_{\Phi_{11}}(t) - \varepsilon_{\Phi_{11}}(t)\right\} \pm \det\left\{z_{\Phi_{11}}(t)\right\}\right)\varphi(t)\,z_A^{\mathrm{T}}(t) - \\ -z_{\Phi_{21}}(t)\,adj\left\{z_{\Phi_{11}}(t)\right\} z_B(t)\,R^{-1}z_B^{\mathrm{T}}(t) - \\ -z_{\Phi_{21}}(t)\,adj\left\{-\varepsilon_{\Phi_{11}}(t)\right\} z_B(t)\,R^{-1}z_B^{\mathrm{T}}(t) + \\ +\varepsilon_{\Phi_{21}}(t)\,adj\left\{\Delta_\Phi(t)\,\Phi_{11}\left(\tau_\infty\right)\right\} z_B(t)\,R^{-1}z_B^{\mathrm{T}}(t) \end{array} \right\} = \\
= \det\left\{ \begin{array}{c} \det\left\{z_{\Phi_{11}}(t)\right\}\varphi(t)\,z_A^{\mathrm{T}}(t) - \\ -z_{\Phi_{21}}(t)\,adj\left\{z_{\Phi_{11}}(t)\right\} z_B(t)\,R^{-1}z_B^{\mathrm{T}}(t) + \\ +\left(\det\left\{z_{\Phi_{11}}(t) - \varepsilon_{\Phi_{11}}(t)\right\} - \det\left\{z_{\Phi_{11}}(t)\right\}\right)\varphi(t)\,z_A^{\mathrm{T}}(t) - \\ -z_{\Phi_{21}}(t)\,adj\left\{-\varepsilon_{\Phi_{11}}(t)\right\} z_B(t)\,R^{-1}z_B^{\mathrm{T}}(t) + \\ +\varepsilon_{\Phi_{21}}(t)\,adj\left\{\Delta_\Phi(t)\,\Phi_{11}\left(\tau_\infty\right)\right\} z_B(t)\,R^{-1}z_B^{\mathrm{T}}(t) \end{array} \right\} \pm \\
\pm \det\left\{\det\left\{z_{\Phi_{11}}(t)\right\}\varphi(t)\,z_A^{\mathrm{T}}(t) - z_{\Phi_{21}}(t)\,adj\left\{z_{\Phi_{11}}(t)\right\} z_B(t)\,R^{-1}z_B^{\mathrm{T}}(t)\right\} = \\
= \det\left\{ \begin{array}{c} \det\left\{z_{\Phi_{11}}(t)\right\}\varphi(t)\,z_A^{\mathrm{T}}(t) - \\ -z_{\Phi_{21}}(t)\,adj\left\{z_{\Phi_{11}}(t)\right\} z_B(t)\,R^{-1}z_B^{\mathrm{T}}(t) + \\ +\left(\det\left\{z_{\Phi_{11}}(t) - \varepsilon_{\Phi_{11}}(t)\right\} - \det\left\{z_{\Phi_{11}}(t)\right\}\right)\varphi(t)\,z_A^{\mathrm{T}}(t) - \\ -z_{\Phi_{21}}(t)\,adj\left\{-\varepsilon_{\Phi_{11}}(t)\right\} z_B(t)\,R^{-1}z_B^{\mathrm{T}}(t) + \\ +\varepsilon_{\Phi_{21}}(t)\,adj\left\{\Delta_\Phi(t)\,\Phi_{11}\left(\tau_\infty\right)\right\} z_B(t)\,R^{-1}z_B^{\mathrm{T}}(t) \end{array} \right\} - \\
- \det\left\{\det\left\{z_{\Phi_{11}}(t)\right\}\varphi(t)\,z_A^{\mathrm{T}}(t) - z_{\Phi_{21}}(t)\,adj\left\{z_{\Phi_{11}}(t)\right\} z_B(t)\,R^{-1}z_B^{\mathrm{T}}(t)\right\} + \\
+ \det\left\{\det\left\{z_{\Phi_{11}}(t)\right\}\varphi(t)\,z_A^{\mathrm{T}}(t) - z_{\Phi_{21}}(t)\,adj\left\{z_{\Phi_{11}}(t)\right\} z_B(t)\,R^{-1}z_B^{\mathrm{T}}(t)\right\}
\end{array}
\tag{S11}
$$

Considering the final expression of $\Delta_{K_r}(t)$, the summonds highlighted in blue are $\Delta_{K_r}(t)$ exactly, whereas the ones highlighted in red will be used to form $\varepsilon_{K_r}(t)$. Then it could be written that:

$$
\begin{array}{c}
y_{K_r}(t) = -\varphi(t)\,R^{-1}z_B^{\mathrm{T}}(t)\times \\
\times adj\left\{ \begin{array}{c} \varphi(t)\,z_A^{\mathrm{T}}(t)\det\left\{z_{\Phi_{11}}(t)\right\} - \\ -z_{\Phi_{21}}(t)\,adj\left\{z_{\Phi_{11}}(t)\right\} z_B(t)\,R^{-1}z_B^{\mathrm{T}}(t) \end{array} \right\} z_{\Phi_{21}}(t)\,adj\left\{z_{\Phi_{11}}(t)\right\} B_r = \\
= -\,\varphi(t)\,R^{-1}z_B^{\mathrm{T}}(t)\,adj\left\{ \begin{array}{c} z_A^{\mathrm{T}}(t)\,\Delta_{K_x}(t) + \\ y_{K_x}^{\mathrm{T}}(t)\,z_B^{\mathrm{T}}(t) \end{array} \right\} z_{\Phi_{21}}(t)\,adj\left\{z_{\Phi_{11}}(t)\right\} B_r,
\end{array}
\tag{S12}
$$

$$
\begin{array}{c}
\Delta_{K_r}(t) = \det\left\{ \begin{array}{c} \det\left\{z_{\Phi_{11}}(t)\right\}\varphi(t)\,z_A^{\mathrm{T}}(t) - \\ z_{\Phi_{21}}(t)\,adj\left\{z_{\Phi_{11}}(t)\right\} z_B(t)\,R^{-1}z_B^{\mathrm{T}}(t) \end{array} \right\} = \\
= \det\left\{\Delta_{K_x}(t)\,z_A^{\mathrm{T}}(t) + y_{K_x}^{\mathrm{T}}(t)\,z_B^{\mathrm{T}}(t)\right\},
\end{array}
\tag{S13}
$$

$$
\begin{gathered}
\varepsilon_{K_r}(t) = \det\left\{\det\left\{z_{\Phi_{11}}(t)\right\}\varphi(t)\, z_A^{\mathrm{T}}(t) - \right.\\
-z_{\Phi_{21}}(t)\, adj\left\{z_{\Phi_{11}}(t)\right\} z_B(t)\, R^{-1} z_B^{\mathrm{T}}(t) + \\
+\left(\det\left\{z_{\Phi_{11}}(t) - \varepsilon_{\Phi_{11}}(t)\right\} - \det\left\{z_{\Phi_{11}}(t)\right\}\right)\varphi(t)\, z_A^{\mathrm{T}}(t) - \\
-z_{\Phi_{21}}(t)\, adj\left\{-\varepsilon_{\Phi_{11}}(t)\right\} z_B(t)\, R^{-1} z_B^{\mathrm{T}}(t) + \\
\left. + \varepsilon_{\Phi_{21}}(t)\, adj\left\{\Delta_\Phi(t)\,\Phi_{11}\left(\tau_\infty\right)\right\} z_B(t)\, R^{-1} z_B^{\mathrm{T}}(t)\right\} K_r - \\
-\det\left\{\begin{array}{l} \det\left\{z_{\Phi_{11}}(t)\right\}\varphi(t)\, z_A^{\mathrm{T}}(t) - \\ -z_{\Phi_{21}}(t)\, adj\left\{z_{\Phi_{11}}(t)\right\} z_B(t)\, R^{-1} z_B^{\mathrm{T}}(t) \end{array}\right\} K_r - \\
-\varphi(t)\, R^{-1} z_B^{\mathrm{T}}(t) \times \\
\times adj\left\{\begin{array}{l} \varphi(t)\, z_A^{\mathrm{T}}(t) \det\left\{\Delta_\Phi(t)\,\Phi_{11}\left(\tau_\infty\right)\right\} - \\ -\Delta_\Phi(t)\,\Phi_{21}\left(\tau_\infty\right) adj\left\{\Delta_\Phi(t)\,\Phi_{11}\left(\tau_\infty\right)\right\} z_B(t)\, R^{-1} z_B^{\mathrm{T}}(t) \end{array}\right\} \times \\
\times \varepsilon_{\Phi_{21}}(t)\, adj\left\{\Delta_\Phi(t)\,\Phi_{11}\left(\tau_\infty\right)\right\} B_r + \varphi(t)\, R^{-1} z_B^{\mathrm{T}}(t) \times \\
\times adj\left\{\begin{array}{l} \varphi(t)\, z_A^{\mathrm{T}}(t) \det\left\{\Delta_\Phi(t)\,\Phi_{11}\left(\tau_\infty\right)\right\} - \\ -\Delta_\Phi(t)\,\Phi_{21}\left(\tau_\infty\right) adj\left\{\Delta_\Phi(t)\,\Phi_{11}\left(\tau_\infty\right)\right\} z_B(t)\, R^{-1} z_B^{\mathrm{T}}(t) \end{array}\right\} \times \\
\times z_{\Phi_{21}}(t)\, adj\left\{-\varepsilon_{\Phi_{11}}(t)\right\} B_r + \varphi(t)\, R^{-1} z_B^{\mathrm{T}}(t) \times \\
\times adj\left\{\varepsilon_{\Phi_{21}}(t)\, adj\left\{\Delta_\Phi(t)\,\Phi_{11}\left(\tau_\infty\right)\right\} z_B(t)\, R^{-1} z_B^{\mathrm{T}}(t)\right\} \times \\
\times z_{\Phi_{21}}(t)\, adj\left\{z_{\Phi_{11}}(t)\right\} B_r + \\
+\varphi(t)\, R^{-1} z_B^{\mathrm{T}}(t)\, adj\left\{-z_{\Phi_{21}}(t)\, adj\left\{-\varepsilon_{\Phi_{11}}(t)\right\} z_B(t)\, R^{-1} z_B^{\mathrm{T}}(t)\right\} \times \\
\times z_{\Phi_{21}}(t)\, adj\left\{z_{\Phi_{11}}(t)\right\} B_r + \varphi(t)\, R^{-1} z_B^{\mathrm{T}}(t) \times \\
\times adj\left\{\varphi(t)\, z_A^{\mathrm{T}}(t)\left(\det\left\{z_{\Phi_{11}}(t) - \varepsilon_{\Phi_{11}}(t)\right\} - \det\left\{z_{\Phi_{11}}(t)\right\}\right)\right\} \times \\
\times z_{\Phi_{21}}(t)\, adj\left\{z_{\Phi_{11}}(t)\right\} B_r .
\end{gathered} \tag{S14}
$$

which are exactly the final equations of $y_{K_r}(t)$, $\Delta_{K_r}(t)$ and $\varepsilon_{K_r}(t)$ in (A7) in the manuscript.

## ACKNOWLEDGMENTS

This research was financially supported by Grants Council of the President of the Russian Federation (project MD-1787.2022.4).

□
